# Supplementary material for: Data-Driven Gain Scheduling Control of Linear Parameter-Varying Systems using Quadratic Matrix Inequalities
Source: arXiv:2209.06251 source file (2022-12-03)
Supplement: Supplementary file 1 [file appendix_h2_norm.tex]

\newpage
\appendix
\section{H2 norm for LPV systems}
\urg{Mario wrote this for our personal reference, this is not going in the 6-page paper}
\MS{This is the new version consistent with the definition of $H_2$ norm as the worst case value over all parameter trajectories of the  expected root-mean-square (RMS) value of the output when the input is a  unit variance white noise process.}

Given the system
\begin{align}
    x^+ &= \textstyle A(\theta) x  + F w  \nonumber \\
    z &= C x \label{eq:h2_sys_app}
\end{align}
  Given a fixed parameter trajectory $\theta_k$, denote by $\phi_k$ the corresponding transition matrix at time $k$, e.g. $\phi_0=I, \phi_1 =A(\theta_1), \phi_2 =A(\theta_2)A(\theta_1)\ldots, \phi_k = \prod_{i=1}^k A(\theta_{k+1-i})$. 
  \subsection{Continuous time case}
  
  The  output corresponding to a given parameter  trajectory and  input $w$ is
   \begin{equation}\label{eq:z20}
   z(t)=C\int_{0}^t \phi(t,\tau)Fw(\tau)d\tau
   \end{equation}
   where $\phi(t,\tau)$ is the transition matrix corresponding to $A[\rho(t)]$. Hence
   \begin{equation}\label{eq:z21}
   \begin{aligned}
  & \|z(t)\|^2 =\textrm{Trace}(zz^T)\\ &=\textrm{Trace}\left (C \int_{0}^t \int_{0}^t \phi(t,\tau)Fw(\tau)w^T(\sigma)F^T\phi^T(t,\sigma)d\tau d\sigma C^T \right)
   \end{aligned}
   \end{equation}
   Hence
    \begin{equation}\label{eq:Ez}
    \mathcal{E}\|z(t)\|^2=
    \textrm{Trace}\left (C \int_{0}^t  \phi(t,\tau)FF^T\phi^T(t,
    \tau)d\tau C^T \right)
     \end{equation}
     where we used the fact that $\mathcal{E}(w(\tau)w^T(\sigma))=\delta(\tau-\sigma)I$. 
     \begin{thm}
     Assume that there exist a matrix $M\succ 0$ such that for all $A(t)$ the following holds:
  \begin{equation}\label{eq:M}   A(t)M+MA(t) \preceq -FF^T
  \end{equation}
  Then 
  \[ \frac{1}{T}\mathcal{E} \int_0^T \|z\|^2 \leq \textrm{Trace}(C^TMC) \]
  \end{thm}
  \begin{proof}
  From \eqref{eq:Ez} we have that 
   \begin{equation}\label{eq:proof1}
   \begin{aligned}
  &   \mathcal{E}\|z(t)\|^2=
    \textrm{Trace}\left (C \int_{0}^t  \phi(t,\tau)FF^T\phi^T(t,
    \tau)d\tau C^T \right) \\
    & \leq \textrm{Trace}\left (C \int_{0}^t  \phi(t,\tau)(-AM-MA)\phi^T(t,
    \tau)d\tau C^T \right) \\
    &= \textrm{Trace}\left (C \int_{0}^t \frac{d}{d\tau} \left [\phi(t,\tau)M\phi^T(t,\tau\right])d\tau C^T\right) \\
    & \leq {Trace}\left (CMC^T \right ) \Rightarrow   \frac{1}{T}\mathcal{E} \int_0^T \|z\|^2 \leq \textrm{Trace}(C^TMC)
   \end{aligned} 
   \end{equation}
  \end{proof}
\begin{cor} For LPVA systems, the $H_2$ norm is bounded above by
\[\begin{aligned}&\|G\|_2^2 \leq \min_{M\succeq 0}\textrm{Trace}(C^TMC) \; \text{subject to} \\
& A_vM+MA_v \preceq -FF^T, \; v=1,\ldots,n_v
\end{aligned} \]
\end{cor}

\subsection{Discrete time case}
  
  In this case, the  output corresponding to a given parameter  trajectory and  input $w$ is
   \begin{equation}\label{eq:z20}
   z(k)=C\sum_{i=0}^k \phi(k,i)Fw(i)
   \end{equation}
   where $\phi(k,i$ is the transition matrix corresponding to $A[\rho(k)]$. Proceeding as in the continuous time case and using the fact that
   $\mathcal{E}(w(k)w^T(i)= \delta_{i,k}I$ and that the system is strictly proper we have 
  
    \begin{equation}\label{eq:dEz}
    \mathcal{E}\|z(k)\|^2=
    \textrm{Trace}\left (C \sum_{i=1}^k  \phi(k,i)FF^T\phi^T(k,i) C^T \right); \; k \geq 1
     \end{equation}
    
     \begin{thm}
     Assume that there exist a matrix $M\succ 0$ such that for all $A(k)$ the following holds:
  \begin{equation}\label{eq:dM}   A(k)MA^T(k)-M \preceq -FF^T
  \end{equation}
  Then 
  \[ \frac{1}{N}\mathcal{E} \sum_0^N \|z\|^2 \leq \textrm{Trace}(C^TMC) \]
  \end{thm}
  \begin{proof}
  From \eqref{eq:Ez} we have that 
   \begin{equation}\label{eq:proofd1}
   \begin{aligned}
  &   \mathcal{E}\|z(t)\|^2=
    \textrm{Trace}\left (C \sum_{i=1}^t  \phi(t,i)FF^T\phi^T(t,
    i)C^T \right) \\
    & \leq \textrm{Trace}\left (C \sum_{i=1}^t  \phi(t,i)(-A(i-1)MA^T(i-1)+M)\phi^T(t,i)d C^T \right) \\
    &= \textrm{Trace}\left (C \left (\sum_{i=0}^{t-1} - \phi(t,i)M\phi^T(t,i) + \sum_{i=1}^t \phi(t,i)M\phi^T(t,i) \right ) C^T\right) \\
    & \leq {Trace}\left (CMC^T \right ) \Rightarrow   \frac{1}{N}\mathcal{E} \sum_1^N \|z\|^2 \leq \textrm{Trace}(C^TMC)
   \end{aligned} 
   \end{equation}
  \end{proof}
  
\begin{cor} For discrete time LPVA systems, the $H_2$ norm is bounded above by
\[\begin{aligned}&\|G\|_2^2 \leq \min_{M\succeq 0}\textrm{Trace}(C^TMC) \; \text{subject to} \\
& A_vMA^T_v -M \preceq -FF^T, \; v=1,\ldots,n_v
\end{aligned} \]
\end{cor}
